# Supplementary material for: Smoke: Fine-grained Lineage at Interactive Speed
Source: arXiv:1801.07237 source file (2018-01-22)
Supplement: Supplementary file 1 [file exp_appendix.tex]

\begin{figure}[h]
\centering
\includegraphics[width=\columnwidth]{exp/micro/agg/agg_overhead.png}
\caption{\small Comparison of \sys with logical and physical systems. \sysi and \sysd outperform logical and physical alternatives while incurring low overhead with respect to \sysn.}
\label{fig:gagg_overhead}
\end{figure}

\begin{figure}[h]
\centering
\includegraphics[width=\columnwidth]{exp/micro/agg/lquery.png}
\caption{\small Comparison of \sysl with \sysn for backward lineage queries. Even in this simple case where \sysn scans a narrow table and evaluates an equality with a single integer, \sysl outperforms \sysn across the vast majority of backward lineage queries by large margins. Also, \sysl brings the majority of lineage queries under the important interactivity level of 1ms, with \sysn being over 20 ms.}
\label{fig:lquery}
\end{figure}

\section{Microbenchmarks}
\label{ss:exp:micro}
In this section, we present a set of controlled microbenchmarks for single operators including group-by aggregation (\Cref{sss:exp:micro:gagg}), PkFk joins (\Cref{sss:exp:micro:pkfk}), m:n joins (\Cref{sss:exp:micro:mnjoins}), and selections (\Cref{sss:exp:micro:selection}).

\subsection{Group-by Aggregation}
\label{sss:exp:micro:gagg}
To evaluate lineage capture techniques for the aggregation operator we use the following group-by aggregation query:
{
\begin{lstlisting}[
	language = SQL,
	showspaces=false,
	basicstyle=\ttfamily,
	commentstyle=\color{gray},
	mathescape=true,
	numbers=none,
	frame = none,
    escapeinside={<}{>},
    label={dl:lsql1}
 		]
SELECT    z, COUNT(*), SUM(v), SUM(v*v),
          SUM(sqrt(v)), MIN(v), MAX(v) 
FROM      zipf 
GROUP BY  z -- #groups follow a zipfian
\end{lstlisting}
}
\noindent This query computes multiple statistics over the attribute \texttt{v} of the table \texttt{zipf} that we introduced in~\Cref{s:settings}. This type of queries are common in interactive visualizations where multiple statistics and aggregates are combined to avoid redundant scans~\cite{tableau:2015:improving}. Furthermore, it allows us to control our experiments by varying the dataset size, the number of groups, the $\theta$ of the zipfian, and the number of aggregates in the output.

\Cref{fig:gagg_overhead} compares the query latency for the different lineage capture techniques techniques that we introduced in~\Cref{s:settings}. Next, we describe these comparisons in more detail.

\stitle{Comparison with \texttt{Logical} systems. }  Perm's rewrite rule for the aggregation operator joins the output of the aggregation with the input to derive the denormalized form of the lineage graph as a single relation. Using this rewrite rule we derived the \lgerids and \lgefull techniques that we described in~\Cref{s:settings}. As shown in~\Cref{fig:gagg_overhead}, these techniques incur an order of magnitude higher lineage capture overheads in contrast to our \sys techniques. The main bottleneck of these approaches is that they need to store the whole denormalized lineage graph, and therefore, incur high capture overheads due to the high redundancy of the denormalization, as we discussed in~\Cref{s:bg}. Finally, note that in these experiments we did not include \lgei because it performs similarly to \lgerids and \lgefull, as we also saw with multiple operators~\Cref{ss:exp:multi}.

\stitle{Comparison with \texttt{Physical} systems. } ~\Cref{fig:gagg_overhead} also shows that our techniques incur lower lineage capture overhead from the physical alternatives \phvfdp and \phbdb. \phvfdp incurs higher overhead because of (a) the virtual emit function calls and (b) the probing of its internal hash table that could be avoided by reusing the hash table generated for the group-by aggregation. In contrast, our techniques avoid these two caveats using tight integration. Furthermore, \phbdb incurs a massive 75X to 250X because of the lineage encoding and indexing of BerkeleyDB and has the worst performance across techniques.  Finally, as we discussed in~\Cref{s:settings}, these results are not intrinsic to group-by aggregation only but rather for all operators, and we avoid further comparisons with physical alternatives.

\stitle{Comparison of \sysl with \sysn for backward lineage query. }~\Cref{fig:lquery} shows the comparion of \sysl with \sysn for backward lineage queries that each traces backwards a single output of the group-by aggregation. For this experiment we used 5000 groups, 10 million records, and we varied $\alpha$ across the values of~\Cref{tab:par}. Even in this extremely simple case, where \sysn needs to evaluate an equality with a single integer, \sysn does not drop the latency below the important interactivity level of 10ms. Under scaling the number of records, having wider input tables, or selections with more sophisticated group-by keys such simple scans cannot compete with \sysl.

\stitle{Varying dataset size, $\theta$, and groups.}
An interesting observation from~\Cref{fig:gagg_overhead} is that all approaches add a constant per-tuple overhead for lineage capture. Hence, increasing the dataset size has a constant impact to lineage overhead which is proportional to the dataset size. Furthermore, varying the parameter $\theta$ of the zipfian does not have an effect on the lineage capture overheads. Finally, increasing the number of groups increases the latency for all lineage capture approaches but also the latency of \sysn. Hence, in our experiments, the relative overheads per technique fluctuated, while varying the number of groups, but remained pairwise the same. 

\stitle{Varying the complexity of group-by keys and aggregate functions.} Another observation is that lineage capture overheads across techniques heavily depend on the input data size and not on the semantics of the group-by aggregation. For instance, if the group-by aggregation computed only a single aggregate, that would require the same lineage capture latency with the one for the current query that computes six aggregates. The reason why is that lineage capture techniques still need to generate the same lineage indexes whose complexity depends only on the input size. Similarly, if the group-by keys become more complex than a single integer, that we use in the current experiment, or we seek to compute more complex aggregates, then again \sysi would require the same time to generate the indexes. This is not the case however for \sysd and logical techniques because they need to join the input with the output on the group-by keys. Hence, the more wide the group-by keys the more the overhead for these approaches.

\stitle{Impact of known cardinalities. } So far, we compared \sysi with alternatives without using the optimization that we discussed in~\Cref{ss:instr} that pre-allocates backward and forward indexes using known cardinalities. The availability of known cardinalities decreased the lineage capture overhead by 52\%, across our experiments, and the average relative overhead to 0.3X from 0.7X for \sysi.

\subsection{PkFk Join}
\label{sss:exp:micro:pkfk}

\begin{figure}[t]
\centering
\includegraphics[width=\columnwidth]{exp/micro/joinpkfk/pkfk_overhead.png}
\caption{\small Comparison of lineage capture techniques for pk-fk joins.}
\label{fig:pkfk_time_overhead}
\end{figure}

We continue with the set of microbenchmarks for the case of primary key-foreign key joins. To evaluate the lineage capture techniques for this operator we experiment with the following simple pk-fk join query:\lstinline|SELECT * FROM gids, zipf WHERE gids.id = zipf.z|. \texttt{gids} is a table that stores the unique group ids that appear in the zipfian attribute \texttt{z} of \texttt{zipf}. Hence, \texttt{zipf.gid} is a foreign key to \texttt{gids.id} and the number of matches for each \texttt{gids.id} in the join output is governed by the zipfian distribution that \texttt{zipf.z} follows.

\stitle{Comparison with logical techniques. } ~\Cref{fig:pkfk_time_overhead} shows the latency of \sysi in comparison to \lgei, that we introduced in~\Cref{s:settings}, and \sysn. \sysi manages to outperform \lgei because it does not require to annotate the join output followed by an extra step to index and project out annotations, that \lgei needs to perform.  Furthermore, the overhead over \sysn remains negligible to 0.41X on average across our experiments. However, we observed an increase of the per case overhead while increasing the number of groups and the dataset size due to the increase in reallocations that \sysi needs to perform.

\stitle{Impact of known join selectivities. } To avoid the multiple reallocations, as we noted in~\Cref{ss:instr}, our techniques can use join selectivities to pre-allocate space for our lineage indexes.~\Cref{fig:joinpkfk_time_overhead} shows the lineage capture overhead using exact join selectivities (i.e., \textsc{Smoke-I+C}) in comparison to \sysi and \sysn. \textsc{Smoke-I+C} further decreases the capture to 0.23X on average across our experiments from 0.41X of \sysi. Finally, the decrease becomes bigger while we increase the number of groups and dataset size because these cases were most affected by the multiple reallocations. Note that for the case of PkFk joins, the cardinalities for all backward indexes and the forward index of the right table are known, as we discussed in~\Cref{ss:join}. Hence, the reduction of overhead in this experiment is attributed to the reduction of reallocations for the forward index of the left table.

\begin{figure}[t]
\centering
\includegraphics[width=\columnwidth]{exp/micro/joinpkfk/pkfk_cardinalities.png}
\caption{\small Comparison of optimizations for pk-fk joins.}
\label{fig:joinpkfk_time_overhead}
\end{figure}

\smallskip 

So far, we have shown the two main deficiencies of logical lineage capture that \sys avoids: (a) overheads due to capturing the denormalized lineage graph and (b) indexing annotated relations. Next, we present our results for the optimization of m:n joins and selections for which we only report the overheads of our \sys techniques. 

\pagebreak

\subsection{M:N joins}
\label{sss:exp:micro:mnjoins}
For the case of M:N joins, we have set up a benchmark to showcase the impact of the optimizations that we discussed in~\Cref{ss:join}. The query that we experiment with joins two \texttt{zipf} tables on the attribute \texttt{z} that follows the zipfian distribution: \lstinline|SELECT * FROM zipf1,zipf2 WHERE zipf1.z = zipf2.z|.Such queries have high fan-out depending on the number of groups of the zipfian and the number of records per group.

~\Cref{fig:mnjoin_overhead} shows the overhead incurred by \sysi in comparison to the optimization technique that we presented in~\Cref{ss:join}: (a) build only the forward indexes (i.e., \textsc{Smoke-I-Opt-F}) and (b) build both forward and backward indexes (i.e., \textsc{Smoke-I-Opt-BF}) for the left table of the join outside of the probing loop. More specifically, in~\Cref{fig:mnjoin_overhead} we vary the number of groups in the left table of the corresponding hash join to 10 (left chart of~\Cref{fig:mnjoin_overhead}) and 100 (right chart of~\Cref{fig:mnjoin_overhead}). In addition, we vary the number of records in the right table from $10^3$ to $10^5$ (x-axis of~\Cref{fig:mnjoin_overhead}). Furthermore,  we fix the number of records of the left table to 1000 and the groups in the right table to 100. Finally, we do not include the materialization cost of the output relations.

\stitle{Comparison of optimizations for M:N joins. } It is clear from~\Cref{fig:mnjoin_overhead} that the optimizations that we presented in~\Cref{ss:join} decrease even further the lineage capture overhead. Constructing the forward lineage within the probing loop results in multiple reallocations that are expensive. In contrast, generating the forward index outside of the probing loop, using our optimization, comes with knowning the cardinalities for each join match and as a result we incur less reallocations. This is why, in~\Cref{fig:mnjoin_overhead}, \textsc{Smoke-I-OPT-F} outperforms \sysi substantially. Furthermore, an extra benefit comes from pushing outside of the probing loop the construction of the backward lineage index for the left table. This is because the size of the output and the size of the backward index is known outside of the probing loop, and we avoid reallocations by fixing the size of the backward index.

\begin{figure}[t]
\centering
\includegraphics[width=\columnwidth]{exp/micro/mnjoin/mnjoin.png}
\caption{\small Comparison of optimizations for m:n joins.}
\label{fig:mnjoin_overhead}
\end{figure}

\stitle{Varying number of groups. } Finally, it is interesting to see that the lineage capture overhead can decrease with the increase of the number of groups if (a) we fix the size of the left table and (b) the groups of the left table join with the most frequent groups of the right table. In this experiment, the 10 groups of the left table join with the 10 most frequent groups of the right table. This join is larger than the join between the 100 groups of the left table with the 100 groups of the right table. This results in higher lineage capture overhead because we need to create indexes for larger output relations.

\subsection{Selection}
\label{sss:exp:micro:selection}
Finally, we report our results for the case of selections. To evaluate the lineage capture techniques for this operator we experiment with the following selection query: \lstinline|SELECT * FROM zipf WHERE v < ?|. \texttt{v} follows a normal distribution in the range $[0, 100]$, and allows us to specify values for the parameter \texttt{?} with different selectivities. 

\begin{figure}[t]
\centering
\includegraphics[width=\columnwidth]{exp/micro/selection/selection.png}
\caption{\small Comparison of lineage capture techniques for selections.}
\label{fig:selection_overhead}
\end{figure}

~\Cref{fig:selection_overhead} presents the lineage capture latency of \sys 
in comparison to \sysn for one (left chart) and five (right chart)  million records while varying the selectivity. Furthermore, we report results with (i.e., \textsc{Smoke-I+C}) and without (i.e., \sysi) the use of cardinalities, for the pre-allocation of lineage indices, based on the selectivity of the selection. 

\stitle{Comparison of lineage capture techniques for selections. } Across our experiments we observed that the overhead of \sys for selections is neglible. More specifically, \sysi introduces a neglible 0.38X, for one million records, and 0.46X, for five million records, average relative overhead to \sysn across selectivities. Furthermore, using known cardinalities, \textsc{Smoke-I+C} improves over \sysi and decreases the average overhead to 0.14X, for one million records, and 0.15X, for five million records. An interesting note here is that an underestimation of the true selectivities lead to reallocations. Hence, depending on the level of underestimation the average overhead of \textsc{Smoke-I+C} can fluctuate across experiments. Yet, it always performs better than \sysi.
